# Supplementary material for: Generalized Neural Collapse for a Large Number of Classes
Source: arXiv:2310.05351 source file (2023-10-27)
Supplement: Supplementary file 5 [file proof_GNC2.tex]

% \begin{theorem}
% Let $(\mW^\star,\mH^\star)$ be an optimal solution to  \eqref{def:hardmax}. Then, $(\mW^\star,\mH^\star)$ satisfies
% \begin{itemize}[leftmargin=0.22in,topsep=0.2em,itemsep=0.11em]
%     \item {\bf Maximum Margin Spherical Codes (\GNC$_2$)}: $\mW^\star = \argmax\limits_{\mW\in\OB(d,K)} \rho_\onevsrest(\mW)$. 
% \end{itemize}
% \end{theorem}

% \begin{proof}
% To prove the Maximum Margin Spherical Codes (\GNC$_2$), consider the ``HardMax Problem" \eqref{def:hardmax},
% \begin{align*}
% \min_{\W,\H} \quad \max_{i} \max_{k} \max_{k' \neq k} \langle \w_{k'} - \w_{k} , \h_{k,i} \rangle 
% \st \quad \|\vw_k\|_2 = 1, \ \|\vh_{k,i}\|_2 = 1.
% \end{align*}
% According to the within-class variability collapse (\GNC$_1$), we can consider the case of having one sample for each class and get,
% \begin{align*}
% \min_{\W,\H} \quad \max_{k} \max_{k' \neq k} \langle \w_{k'} - \w_{k} , \h_{k} \rangle \quad \st \ \|\vw_k\|_2 = 1, \ \|\vh_{k}\|_2 = 1.
% \end{align*}
% Then according to Theorem \ref{thm:max_min_separation_margin}, we have,
% \begin{align*}
%     \min_{\mW \in\OB(d,K)} \max_{k} \  - \dist(\vw_k,\{\vw_j\}_{j\in[K]\setminus k}),
% \end{align*}
% Since we denote the one-vs-rest margin for the linear classifier $\mW$ in \eqref{eq:margins}, this problem can be written as,
% \begin{align*}
%     \min_{\mW \in\OB(d,K)} \rho_\onevsrest(\mW)
% \end{align*}
% \end{proof}
